# Supplementary material for: Cross-inhibition leads to group consensus despite the presence of strongly opinionated minorities and asocial behaviour
Source: arXiv:2211.09531 source file (2023-07-25)
Supplement: Supplementary file 1 [file supp-text.pdf]

# Supplementary text of the article Cross-inhibition leads to group consensus despite the presence of strongly opinionated minorities and asocial behaviour

Andreagiovanni Reina, Raina Zakir, Giulia De Masi, Eliseo Ferrante

## Supplementary Note 1. The two types of noise of the cross-inhibition model

We study the cross-inhibition model subject to two types of noise: noise type 1 and noise type 2. The generic model of Eq. (7) in the main text can be rewritten for the two types of noise as follows. Considering $\sigma$ noise type 1, we get:

$$\begin{cases} \frac{\mathrm{d}x}{\mathrm{d}t} = x(uq_x - yq_y) + \sigma(\frac{u}{2} - x) \\ \frac{\mathrm{d}y}{\mathrm{d}\tau} = y(uq_y - xq_x) + \sigma(\frac{u}{2} - y)\,. \end{cases} \tag{SE1}$$

Instead, considering $\sigma_2$ noise type 2, we get:

$$\begin{cases} \frac{\mathrm{d}x}{\mathrm{d}\tau} = x(uq_x - yq_y) + \sigma_2(y - x) \\ \frac{\mathrm{d}y}{\mathrm{d}\tau} = y(uq_y - xq_x) + \sigma_2(x - y)\,. \end{cases} \tag{SE2}$$

## Supplementary Note 2. Stationary probability distribution

Here, we report the expanded form of Eqs. (17) and (27) in the main text, which describe the stationary probability distribution (SPD) of the voter model and cross-inhibition model, respectively. We report equations for both types of asocial mechanisms, noise and zealotry.

**Voter model with noise.** We first compute a simplified form of the term $\frac{T^{+x}_{x=j}}{T^{-}_{x=j+1}}$ as

$$\frac{T^{+x}_{x=j}}{T^{-}_{x=j+1}} = \frac{\frac{(S-j)(q_x j+\sigma S-\sigma)}{S-1}}{\frac{(j+1)(q_y(S-(j+1))+\sigma S-\sigma))}{S-1}} = \frac{(S-j)(q_x j + \sigma S - \sigma)}{(j+1)(q_y(S-(j+1)) + \sigma S - \sigma))} =$$

$$\frac{(S-j)(q_x j + \sigma S - \sigma)}{(j+1)(q_y(-j+S-1) + \sigma S - \sigma))} = \left(\frac{S-j}{j+1}\right)\left(\frac{q_x j + \sigma S - \sigma}{q_y(-j+S-1) + \sigma S - \sigma)}\right).$$

Therefore, the SPD of the voter model (Eq. (17) in the main text) with noise is

$$P^*_{x=k} = \frac{\prod_{j=0}^{k-1}\left(\frac{S-j}{j+1}\right)\left(\frac{q_x j+\sigma S-\sigma}{q_y(-j+S-1)+\sigma S-\sigma)}\right)}{1 + \sum_{k=1}^{S-2S_Z}\prod_{j=0}^{k-1}\left(\frac{S-j}{j+1}\right)\left(\frac{q_x j+\sigma S-\sigma}{q_y(-j+S-1)+\sigma S-\sigma)}\right)}.$$

**Voter model with zealots.** We first compute a simplified form of the term $\frac{T^{+x}_{x=j}}{T^{-}_{x=j+1}}$ as

$$\frac{T^{+x}_{x=j}}{T^{-x}_{x=j+1}} = \frac{\frac{q_x(j+S_Z)(S-j-2S_Z)}{S-1}}{\frac{q_y(j+1)(S-(j+1)-2S_Z+S_Z)}{S-1}} = \left(\frac{j+S_Z}{j+1}\right)\left(\frac{q_x(S-j-2S_Z)}{q_y(S-j-1-2S_Z+S_Z)}\right).$$

Therefore, the SPD of the voter model (Eq. (17) in the main text) with zealots is

$$P^*_{x=k} = \frac{\prod_{j=0}^{k-1}\left(\frac{j+S_Z}{j+1}\right)\left(\frac{q_x(S-j-2S_Z)}{q_y(S-j-1-2S_Z+S_Z)}\right)}{1 + \sum_{k=1}^{S-2S_Z}\prod_{j=0}^{k-1}\left(\frac{j+S_Z}{j+1}\right)\left(\frac{q_x(S-j-2S_Z)}{q_y(S-j-1-2S_Z+S_Z)}\right)}.$$

**Cross-inhibition model with noise.** We first compute a simplified form of the terms $\frac{T^{+y}_{x=a,y=b}}{T^{-y}_{x=a,y=b+1}}$, $\frac{T^{+x}_{x=a,y=0}}{T^{-x}_{x=a+1,y=0}}$, and $\frac{T^{+y}_{x=0,y=b}}{T^{-y}_{x=0,y=b+1}}$ as

$$\frac{T^{+y}_{x=a,y=b}}{T^{-y}_{x=a,y=b+1}} = \frac{\frac{(S-a-b)(q_y b+\sigma(S-1))}{S-1}}{\frac{(b+1)(q_x a+\sigma(S-1))}{S-1}} = \frac{(S-a-b)(q_y b+\sigma(S-1))}{(b+1)(q_x a+\sigma(S-1))} = \left(\frac{S-a-b}{b+1}\right)\left(\frac{q_y b+\sigma S-\sigma}{q_x a+\sigma S-\sigma}\right).$$

$$\frac{T^{+x}_{x=a,y=0}}{T^{-x}_{x=a+1,y=0}} = \frac{\frac{(S-a)(q_x a+\sigma(S-1))}{S-1}}{\frac{(a+1)(q_y+\sigma(S-1))}{S-1}} = \frac{(S-a)(q_x a+\sigma(S-1))}{(a+1)(q_y+\sigma(S-1))} = \left(\frac{S-a}{a+1}\right)\left(\frac{q_x a+\sigma S-\sigma}{q_y+\sigma S-\sigma}\right).$$

$$\frac{T^{+y}_{x=0,y=b}}{T^{-y}_{x=0,y=b+1}} = \frac{\frac{(S-b)(q_y b+\sigma(S-1))}{S-1}}{\frac{(b+1)(q_x+\sigma(S-1))}{S-1}} = \frac{(S-b)(q_y b+\sigma(S-1))}{(b+1)(q_x+\sigma(S-1))} = \left(\frac{S-b}{b+1}\right)\left(\frac{q_y b+\sigma S-\sigma}{q_x+\sigma S-\sigma}\right).$$

The SPD of the cross-inhibition model (Eq. (27) in the main text) with noise type 1 is

$$\frac{\prod_{j=0}^{a-1}\left(\frac{S-j}{j+1}\right)\left(\frac{q_x j+\sigma S-\sigma}{q_y+\sigma S-\sigma}\right)\prod_{j=0}^{b-1}\left(\frac{S-a-j}{j+1}\right)\left(\frac{q_y j+\sigma S-\sigma}{q_x a+\sigma S-\sigma}\right)}{1+\sum_{b=1}^{S}\prod_{j=0}^{b-1}\left(\frac{S-j}{j+1}\right)\left(\frac{q_y j+\sigma S-\sigma}{q_x+\sigma S-\sigma}\right)+\sum_{a=1}^{S}\prod_{j=0}^{a-1}\left(\frac{S-j}{j+1}\right)\left(\frac{q_x j+\sigma S-\sigma}{q_y+1+\sigma S-\sigma}\right)\left(1+\sum_{b=1}^{(S-a)}\prod_{k=0}^{b-1}\left(\frac{S-a-k}{k+1}\right)\left(\frac{q_y k+\sigma S-\sigma}{q_x a+\sigma S-\sigma}\right)\right)}.$$

**Cross-inhibition model with zealots.** We first compute a simplified form of the terms $\frac{T^{+y}_{x=a,y=b}}{T^{-y}_{x=a,y=b+1}}$, $\frac{T^{+x}_{x=a,y=0}}{T^{-x}_{x=a+1,y=0}}$, and $\frac{T^{+y}_{x=0,y=b}}{T^{-y}_{x=0,y=b+1}}$ as

$$\frac{T^{+y}_{x=a,y=b}}{T^{-y}_{x=a,y=b+1}} = \frac{\frac{q_y(b+S_Z)(S-a-b-2S_Z)}{S-1}}{\frac{q_x(b+1)(a+S_Z)}{S-1}} = \left(\frac{b+S_Z}{b+1}\right)\left(\frac{q_y(S-a-b-2S_Z)}{q_x(a+S_Z)}\right).$$

$$\frac{T^{+x}_{x=a,y=0}}{T^{-x}_{x=a+1,y=0}} = \frac{\frac{q_x(a+S_Z)(S-a-2S_Z)}{S-1}}{\frac{q_y S_Z(a+1)}{S-1}} = \left(\frac{a+S_Z}{a+1}\right)\left(\frac{q_x(S-a-2S_Z)}{q_y S_Z}\right).$$

$$\frac{T^{+y}_{x=0,y=b}}{T^{-y}_{x=0,y=b+1}} = \frac{\frac{q_y(b+S_Z)(S-b-2S_Z)}{S-1}}{\frac{q_x S_Z(b+1)}{S-1}} = \left(\frac{b+S_Z}{b+1}\right)\left(\frac{q_y(S-b-2S_Z)}{q_x S_Z}\right).$$

The SPD of the cross-inhibition model (Eq. (27) in the main text) with zealots is

$$\frac{\prod_{j=0}^{a-1}\left(\frac{j+S_Z}{j+1}\right)\left(\frac{q_x(S-j-2S_Z)}{q_y S_Z}\right)\prod_{j=0}^{b-1}\left(\frac{j+S_Z}{j+1}\right)\left(\frac{q_y(S-a-j-2S_Z)}{q_x(a+S_Z)}\right)}{1+\sum_{b=1}^{(S-2S_Z)}\prod_{j=0}^{b-1}\left(\frac{j+S_Z}{j+1}\right)\left(\frac{q_y(S-j-2S_Z)}{q_x S_Z}\right)+\sum_{a=1}^{S-2S_Z}\prod_{j=0}^{a-1}\left(\frac{j+S_Z}{j+1}\right)\left(\frac{q_x(S-j-2S_Z)}{q_y S_Z}\right)\left(1+\sum_{b=1}^{(S-2S_Z-a)}\prod_{k=0}^{b-1}\left(\frac{k+S_Z}{k+1}\right)\left(\frac{q_y(S-a-k-2S_Z)}{q_x(a+S_Z)}\right)\right)}.$$

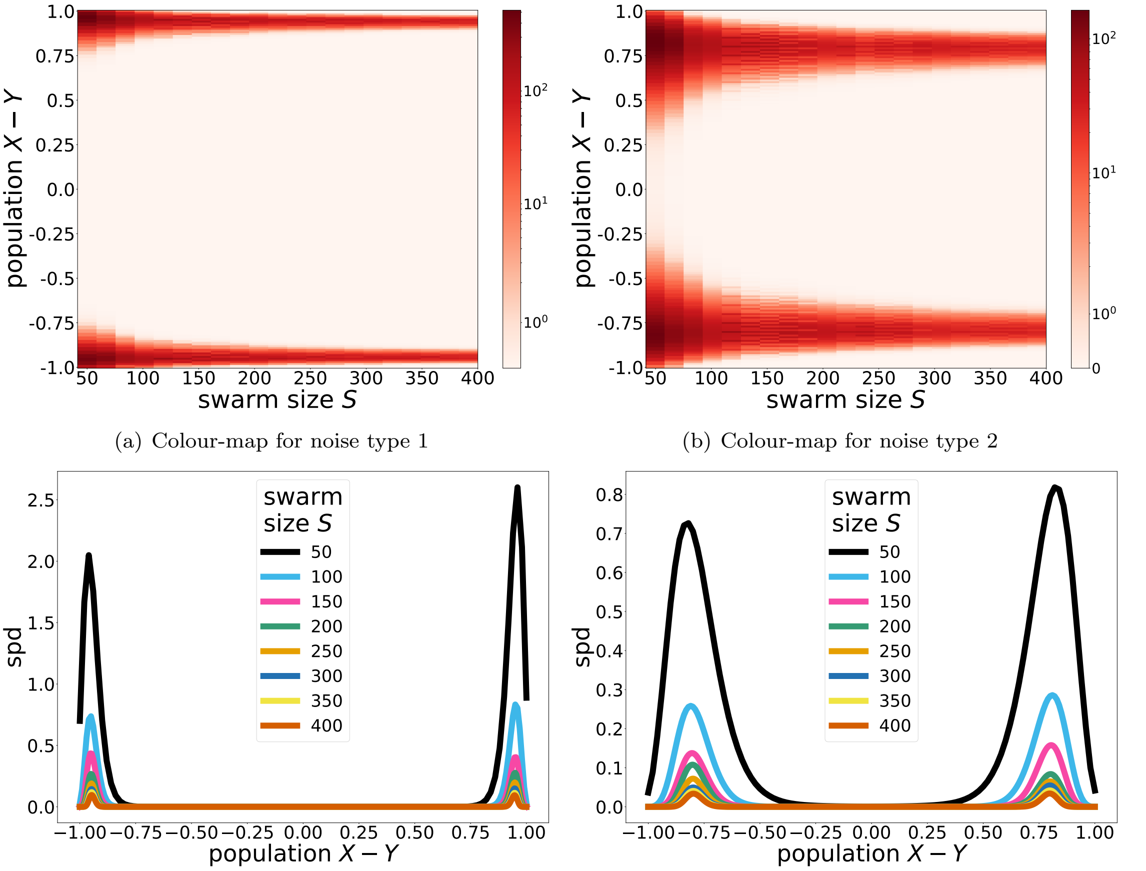


(a) Colour-map for noise type 1

(b) Colour-map for noise type 2

(c) Selected SPD for noise type 1

(d) Selected SPD for noise type 2

Figure S1: On the top row, the red colour-maps show the stationary probability distribution (SPD) computed with the results of $10^3$ Gillespie SSA simulations for various swarm sizes $S \in [50, 400]$ (with values of $S$ increasing on the y-axis). On the bottom row, the two plots show the SPDs computed through Gillespie simulations for seven selected swarm sizes $S$. The bottom-row plots show a subset of the results reported in the colour-maps on the top row. The results are computed for $q = q_x/q_y = 1$ and $\sigma = 0.05$, for the cross-inhibition model with both types of noise: panels (a,c) are the results for noise type 1, and panels (b,d) for noise type 2. For every simulation, we initialise the system with a random initial condition and store the amount of time spent in each state throughout long runs ($10^5$ time-units); finally we normalised the time in each state by the total simulation length. Differently from the direct-switch model, the cross-inhibition model is highly stable regardless of the system size: the system is always bistable (denoted by the two peaks near -1 and +1) for both types of noise.

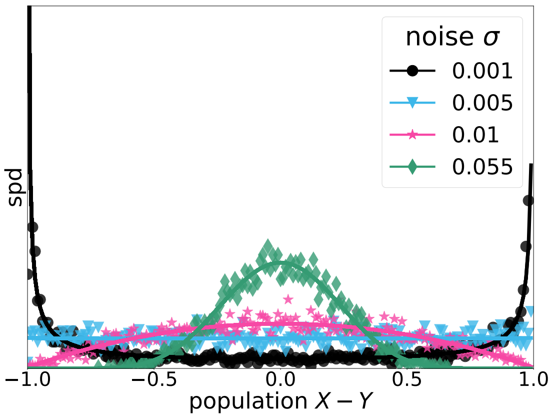


(a) Voter model with noise

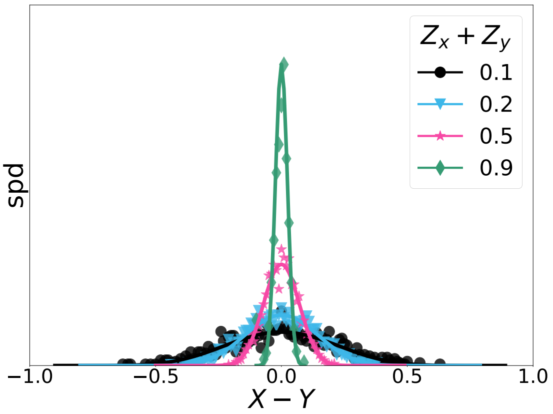


(b) Voter model with zealots

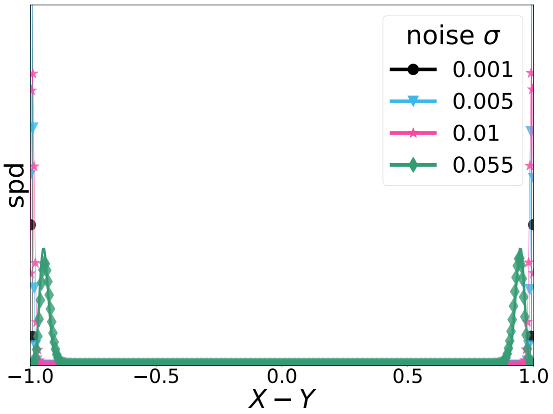


(c) Cross-inhibition with noise

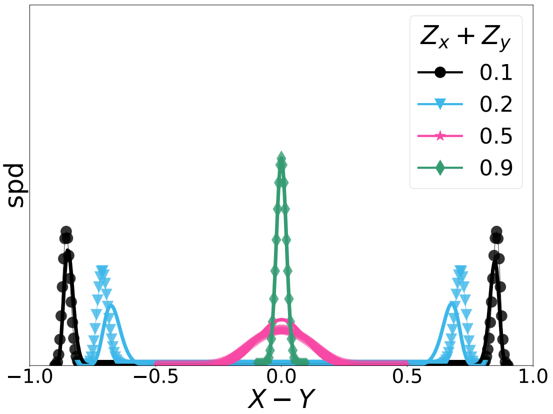


(d) Cross-inhibition with zealots

Figure S2: Comparison of the stationary probability distributions computed using the analytical solution (Eqs. (17) and (27) in the main text) and computed using the Gillespie's SSA algorithm. We report results for $q = q_x/q_y = 1$, for both models—(a-b) the voter model, and (c-d) the cross-inhibition model—and for both asocial mechanisms—(a,c) noise and (b,d) zealots. The lines show the results from the equations, and the markers show the results of $10^3$ Gillespie simulations. For every simulation, we initialise the system with a random initial condition and store the amount of time spend in each state throughout long runs (5x$10^4$ time-units), finally we normalised the time in each state by the total simulation length. The results from Gillespie's SSA approximate well, in all tested conditions, the stationary probability distribution obtained form the equations.
